# Supplementary material for: E-VLC: A Real-World Dataset for Event-based Visible Light Communication And Localization
Source: arXiv:2504.18521 source file (2025-04-25)
Supplement: Supplementary file 1 [file suppl.tex]

\cleardoublepage

\section{Supplementary}
\label{sec:suppl}

\subsection{Video}
We encourage readers to inspect the attached video,
which summarizes the method and the results.

\input{floats/fig_suppl_optimization}

\subsection{Denoising Convergence During Optimization}

To further validate the proposed joint estimation approach,
we analyze the convergence during the joint estimation using the ECD dataset in \cref{fig:suppl:optim} (see also results in \cref{fig:result:angvelComp}).
At the first iteration (i.e., \emph{initialization}),
signal and noise events are classified randomly.
As the optimization proceeds,
signal events evolve to keep edge structures in the scene,
while noise events evolve to drop such edge structures (see the second and third rows).
Also, the IWEs converge to sharp edges with correct motion parameters.
This example further confirms the efficacy of the joint estimation.

\subsection{Full Results on Angular Velocity Estimation}

While the quantitative evaluation on angular velocity estimation is summarized in \cref{fig:result:angvel_quantitative},
here, we report the detailed results with different target ratio parameters, also compared with other baselines such as BA Filter \cite{Delbruck08issle}.
The original CMax degrades due to noise, as reported in previous work (e.g., \cite{Arja23cvprw}).
The S/N target ratio $\snratio$ affects the accuracy:
when it is close to the actual value of noise injection, the result of the proposed method becomes better.
The amount of artificial noise injected is around $15$~\% for $5$~Hz and $3$~\% for $1$~Hz conditions.
Although we cannot know the ``true'' noise level due to the original noise in the ECD sequences,
our method constantly produces better accuracy and FWL than other baselines.
Please refer to \cref{sec:experim:angVel} for more discussions
about dependency on initialization and comparison with other baselines.
The AUCs for the conditions that we test ($\snratio=\{0.9,\ldots,0.7\}$) are $0.70$ (``Ours'') and $0.67$ (``Downsampling'').

\input{floats/tab_result_angvel}

\subsection{Quantitative Evaluation of Intensity Reconstruction}

In \cref{sec:experim:intensityRecon,sec:sensitivity} we show qualitative results of the intensity reconstruction application.
Here, we discuss possible quantitative evaluation.
The challenge of the quantitative evaluation lies in the quality of reference frames (i.e., ``GT'') in the existing dataset as shown in \cref{fig:result:denoiseQuality,fig:result:endRecon}:
the frames become underexposed or blurry due to their limited dynamic range,
when event data suffer from more BA noise (i.e., in dark scenes).

Nonetheless, we report non-reference image quality indices for different S/N ratios ($\snratio$).
\Cref{fig:result:suppl:nriq} reports the scores of
Blind/Referenceless Image Spatial Quality Evaluator (BRISQUE) \cite{Mittal12tip} and
Naturalness Image Quality Evaluator (NIQE)  \cite{Mittal12spl},
using \emph{Bicycle-ND64-2} sequence (same as \cref{fig:sensitivity:recon}).
These scores indicate the perceptual quality of images, and smaller is better.
Although BRISQUE monotonically increases as the target ratio decreases (i.e., more events are removed),
NIQE scores the lowest at $\snratio=0.9$, indicating the best quality of the reconstructed image.
Although the results potentially suggest that it could estimate the ``true'' noise ratio in the data using the non-reference indices, which is useful for image reconstruction applications,
we leave further evaluation and discussion as future work.

\input{floats/fig_suppl_sensitivity_niqe}
